# Supplementary material for: Trade Co-occurrence, Trade Flow Decomposition, and Conditional Order Imbalance in Equity Markets
Source: arXiv:2209.10334 source file (2024-03-13)
Supplement: Supplementary file 1 [file appendix_sharpe.tex]

\section{Imbalance-sorted portfolio analysis}
As discussed in previous sections, there is evidence that conditional order imbalances contain signals for explaining and forecasting individual stock returns. In this section, we exploit their economic values and contribution to portfolio design. To assess economic gains, we first form characteristic-sorted portfolios based upon order imbalance signals. After translating order imbalances into portfolios, we can compare their profits and losses (PnL), which is the daily portfolio return, as well as Sharpe Ratios \cite{sharpe1994sharpe}. Backtests of our strategies, over the entire sample period from 2017-01-01 to 2019-12-11, reinforce our findings in predictive regression. The 'iso' and 'nis-s' imbalances are momentum signals while the 'nis', 'nis-c' and 'nis-b' imbalances are reversal signals. Betting on individual conditional order imbalance generates significant profits. If we incorporate multiple signals, the profits are even better. 

\subsection{Portfolio Construction and Evaluation}
Portfolio sorting (\cite{fama1992cross} \cite{cattaneo2020characteristic}) is a popular method in empirical asset pricing. We modify this technique to form daily rebalanced zero-investment portfolios. The procedure to build a imbalance-sorted portfolio is as follows. 

At each time $t$, there is a cross-section of order imbalances $\rho_{1,t}, \rho_{2,t} \dots, \rho_{457,t}$, where each $\rho_{1,t}$ belongs to stock $i$. Firstly, we sort the order imbalances from low to high with respect to their absolute value. Secondly, we decide the proportion of stocks to include in the portfolio, $P_{a, t}$. Finally we decide the bet size, $b_{j,t}$, and direction, $d_{j,t} \in \{ -1, 1 \}$ (1 = buy and -1 = sell), for each selected stock to invest. Then the daily portfolio PnL in percentage can be calculated as 
\begin{equation*}
    PnL_{a, t} = \frac{\sum_{j \in P_{a,t-1}} d_j b_j R_{j,t}}{\sum_{j \in P_{a,t}} b_{j,t-1}}
\end{equation*}
where $R_{j,t}$ is the open-to-close market excess return of stock $j$ at time $t$.

In this study, we build five portfolios, denoted as Q-20, Q-40, Q-60, Q-80 and Q-100, corresponding to quantile imbalance-sorted portfolios including stocks with top 20$\%$, 40$\%$, 60$\%$, 80$\%$ and 100$\%$ of absolute order imbalance. We only build equally weighted portfolios so that the bet sizes for all stocks in the same portfolio are identical, implying that the $b_{j,t}$ can be set to 1 without losing generality. In addition, all the portfolios are rebalanced every day. Finally, to be consistent with our analysis, we use market excess return to calculate the PnL, which is equivalent to form a self-financing portfolio, $P_{z}$, including the sorted portfolio and an extra market portfolio with same size and opposite direction. The portfolio PnL is then given by 
\begin{equation*}
    PnL_{z,t} := \frac{\sum_{j \in P_{z,t-1}} d_j r_{j,t}}{|P_{z,t-1}|}.
\end{equation*}

Given the portfolios and daily PnL, the annulized Sharpe ratio is defined as
\begin{equation*}
    S_{z} := \frac{\textit{mean }(PnL_{z,t})}{\textit{std }(PnL_{z,t})} \times \sqrt{252}
\end{equation*}
We do not take the risk free rate, which can be ignored over the period of interest, and transaction costs into account. This simplified Sharpe ratio is symmetric. For example, if a portfolio has a high negative Sharpe, then shorting this portfolio leads to a profitable trading strategy.

\subsection{Portfolio Analysis}
\subsubsection{Single-Sorted Portfolios}
Assuming no prior knowledge about interplay between order imbalances and future returns, we choose as direction $d_{j,t} = sgn(\rho_{j,t}^{*,*})$, which means we bet on the sign of selected signals. \Cref{tab:sort_portfolio_sharpe} documents Sharpe ratios of quantile imbalance-sorted portfolios. Focusing on the signs of Sharpe ratios, we can find that sorting by isolated and non-self-isolated imbalances gives rise to positive Sharpe. On the other hand, non-isolated, non-cross-isolated and non-both-isolated portfolios generate negative ratios. These results echo our findings on relations between imbalances and future returns. Moreover, turning to the magnitudes of Sharpe ratios, we discover that decomposing market order flows can explicitly strengthen trading signals. Initially, simply trading on unconditional order imbalances is not a profitable strategy. After separating isolated and non-isolated orders, we obtain clear signals. Q-60 portfolio for isolated volume imbalance achieves the highest Sharpe of 2.64. Comparatively, the performances of non-isolated based portfolios are inferior, which leads to further decomposing. Profits generated by subgroups exceed investing on non-isolated order imbalances solely. Betting on non-cross order imbalances generally create Sharpe ratios with absolute values greater than 2. 

\begin{sidewaystable}[t]
    \caption{\small Summary of single-sorted portfolios}    
    \input{tables/single_sort_portfolio}
    \label{tab:sort_portfolio_sharpe}
\end{sidewaystable}

\begin{figure}[htp]
    \centering
    \includegraphics[width = 1\textwidth, height = 0.4\textheight]{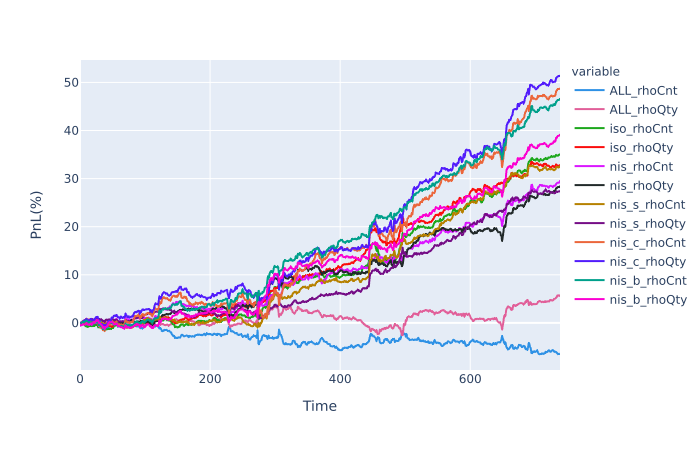}
    \caption{\small  Cumulative Profit $\&$ Loss. This figure plots the Q-20 imbalance-sorted portfolios for each type of order imbalance, over the entire period from 2017 to 2019, encompassing 730 trading days.} 
    \label{fig:pnl_Q20}
\end{figure}

With the signs of relations between types of imbalances and portfolio profitability, we propose to long portfolios of $\rho ^{*, iso}$ and $\rho ^{*, nis-s}$ and to short on $\rho ^{*, nis}$ and $\rho ^{*, nis-c}$, $\rho ^{*, nis-b}$. \Cref{fig:pnl_Q20} provides a visualization of all cumulative PnLs of Q-20 portfolios. From the plot, we can see a clear upwards trend in conditional order imbalances portfolios with minimal fluctuations. Benchmarked by unconditional imbalances, portfolios built upon decomposed trade flows demonstrate conspicuous enhancements on performances.
