# Supplementary material for: Trade Co-occurrence, Trade Flow Decomposition, and Conditional Order Imbalance in Equity Markets
Source: arXiv:2209.10334 source file (2024-03-13)
Supplement: Supplementary file 2 [file appendix_control.tex]

\section{Benchmark regression on control variables} \label{appendix:regression_control}
